# Supplementary material for: SA-Occ: Satellite-Assisted 3D Occupancy Prediction in Real World
Source: arXiv:2503.16399 source file (2025-03-20)
Supplement: Supplementary file 1 [file 12_appendix.tex]

\section{Appendix Section}
\label{sec:appendix_section}
Supplementary material goes here.
